# Supplementary material for: Gradient Obfuscation Gives a False Sense of Security in Federated Learning
Source: arXiv:2206.04055 source file (2022-10-14)
Supplement: Supplementary file 1 [file backup.tex]

% \begin{figure}[!tb]
%     \begin{overpic}[width=\linewidth]{figs/3x4.pdf}
%     \put(17, 46){\includegraphics[width=0.2\linewidth]{figs/appendix/ori_3.png}}
%     \put(38, 46){\includegraphics[width=0.2\linewidth]{figs/appendix/ori_7.png}}
%     \put(59, 46){\includegraphics[width=0.2\linewidth]{figs/appendix/ori_8.png}}
%     \put(80, 46){\includegraphics[width=0.2\linewidth]{figs/appendix/ori_23.png}}

%     \put(17, 44){\includegraphics[width=0.825\linewidth, height=1.3pt]{figs/lines/line.png}}

%     \put(17, 22.){\includegraphics[width=0.2\linewidth]{figs/appendix/corrupt_3.png}}
%     \put(38, 22.){\includegraphics[width=0.2\linewidth]{figs/appendix/corrupt_7.png}}
%     \put(59, 22.){\includegraphics[width=0.2\linewidth]{figs/appendix/corrupt_8.png}}
%     \put(80, 22.){\includegraphics[width=0.2\linewidth]{figs/appendix/corrupt_23.png}}

%     \put(17, 1){\includegraphics[width=0.2\linewidth]{figs/appendix/recon_3.png}}
%     \put(38, 1){\includegraphics[width=0.2\linewidth]{figs/appendix/recon_7.png}}
%     \put(59, 1){\includegraphics[width=0.2\linewidth]{figs/appendix/recon_8.png}}
%     \put(80, 1){\includegraphics[width=0.2\linewidth]{figs/appendix/recon_23.png}}

%     \put(0, 54){\zoom[0.64]{Ground Truth}}
%     \put(0, 32){\zoom{Corrupted}}
%     \put(0, 28){\zoom{Images}}
    
%     \put(0, 14){\zoom{Enhanced}}
%     \put(0, 10){\zoom{Images}}
%     \end{overpic}
%     \vspace*{-20pt}
%     \caption{
%     Synthetic dataset for the postprocessing neural networks.
%     The first row gives the ground truth images, and the second row shows different synthetic corruptions. 
%     The enhanced images on the third row show the qualitative output of the postprocessing neural network, which confirms the generalizability of the postprocessing module.  
%     \label{fig:gan_train}}
% \end{figure}

Next, we provide the simulation results on the random-$k$ sparsification method.
% \begin{Example}
%     In random-$k$ compression~\cite{stich2018sparsified}, the client selects $k$ entries in the gradient uniformly at random and zeros out other components.  
%     We denote this function by $\pfunc_{\text{randk}}$. 
% \end{Example}

% The reconstruction against random-$k$ gradient compression is shown in Figure~\ref{fig:attack_randk}.
% Compared to Top-$k$ compression (Figure~\ref{fig:attack_gradcomp}), the reconstructed results have lower quality even when the sparsity is relatively low.  
% On the other hand, the convergence rate and the model performance of random-$k$ may not be comparable to Top-$k$~\cite{xu2021grace}. 
% This is coherent with the reconstruction results that the Top-$k$ gradients preserve most of the information with respect to the raw data. 

% \begin{figure}[!tb]
%     \begin{overpic}[width=\linewidth]{figs/4x4.pdf}
%     \put(17, 69){\includegraphics[width=0.2\linewidth]{figs/appendix/randomk/50/1_recon.png}}
%     \put(38, 69){\includegraphics[width=0.2\linewidth]{figs/appendix/randomk/50/3_recon.png}}
%     \put(59, 69){\includegraphics[width=0.2\linewidth]{figs/appendix/randomk/50/5_recon.png}}
%     \put(80, 69){\includegraphics[width=0.2\linewidth]{figs/appendix/randomk/50/7_recon.png}}

%     \put(17, 67){\includegraphics[width=0.83\linewidth, height=1.3pt]{figs/lines/line.png}}

%     \put(17, 45){\includegraphics[width=0.2\linewidth]{figs/appendix/randomk/30/1_recon.png}}
%     \put(38, 45){\includegraphics[width=0.2\linewidth]{figs/appendix/randomk/30/3_recon.png}}
%     \put(59, 45){\includegraphics[width=0.2\linewidth]{figs/appendix/randomk/30/5_recon.png}}
%     \put(80, 45){\includegraphics[width=0.2\linewidth]{figs/appendix/randomk/30/7_recon.png}}

%     \put(17, 24){\includegraphics[width=0.2\linewidth]{figs/appendix/randomk/50/1_recon.png}}
%     \put(38, 24){\includegraphics[width=0.2\linewidth]{figs/appendix/randomk/50/3_recon.png}}
%     \put(59, 24){\includegraphics[width=0.2\linewidth]{figs/appendix/randomk/50/5_recon.png}}
%     \put(80, 24){\includegraphics[width=0.2\linewidth]{figs/appendix/randomk/50/7_recon.png}}

%     \put(17, 3){\includegraphics[width=0.2\linewidth]{figs/appendix/randomk/70/1_recon.png}}
%     \put(38, 3){\includegraphics[width=0.2\linewidth]{figs/appendix/randomk/70/3_recon.png}}
%     \put(59, 3){\includegraphics[width=0.2\linewidth]{figs/appendix/randomk/70/5_recon.png}}
%     \put(80, 3){\includegraphics[width=0.2\linewidth]{figs/appendix/randomk/70/7_recon.png}}

%     \put(0, 76){\zoom{Raw Image}}
%     \put(0, 55){\zoom{$\pfunc_{\text{randk}}$ $(0.3)$}}
%     \put(0, 51){\zoom{LPIPS $0.270$}}
%     \put(0, 35.5){\zoom{$\pfunc_{\text{randk}}$ $(0.5)$}}
%     \put(0, 31.5){\zoom{LPIPS $0.401$}}
%     \put(0, 16){\zoom{$\pfunc_{\text{randk}}$ $(0.7)$}}
%     \put(0, 12){\zoom{LPIPS $0.614$}}
%     \end{overpic}
%     \vspace*{-20pt}
%     \caption{
%     Reconstruction against random-$k$ gradient compression with different sparsity parameters. 
%     As the sparsity increases, more information is discarded and the reconstruction quality decreases. 
%     \label{fig:attack_randk}}
% \end{figure}
